# Supplementary material for: Towards a Standardised Performance Evaluation Protocol for Cooperative MARL
Source: arXiv:2209.10485 source file (2022-09-21)
Supplement: Supplementary file 1 [file 9-appendix.tex]

\section{Appendix}

Before we delve into the analysis of the collected data, we define our search methodology and discuss the assumptions made while collecting papers.

\subsection{Filtration of relevant studies}

Following the initial data collection, the dataset was refined to ensure relevance using the following criteria:
\begin{itemize}
    \item The papers must be either peer review conference or journal papers, and published in the English language.
    \item The papers are excluded if they uses a custom environment not publicly available among the MARL benchmarking environments. 
    \item The papers are excluded if they are testing a particular algorithm's skill (e.g., testing robustness in MARL by adding perturbations to the environment \cite{}).
\end{itemize}

\subsection{Annotations}

We annotated the following amount of papers during our data collection:
\begin{table}[hbt!]
  \caption{Number of Papers Annotated During Data Collection Per Year}
  \label{sample-table}
  \centering
  \begin{tabular}{ll}
    \toprule
    Publication Year & Papers Annotated \\
    \midrule
    2015 & 1\\
    2016 & 3 \\
    2017 & 7 \\
    2018 & 5 \\
    2019 & 15 \\
    2020 & 26 \\
    2021 & 43\\
    2022 & 14 \\
    \bottomrule
  \end{tabular}
\end{table}

We annotated each paper as follows:
\begin{enumerate}[label=A{{\arabic*}}.]
\item For the metrics used to evaluate an algorithms performance, we omit overly specialised metrics in papers (e.g., name of special metric and cite paper) and we opt for only recording metrics that are comparable across papers. %Were any of these specialised metrics useful for a rigorous empirical evaluation protocol
\item For the reported metrics, we did not list the variants of the same metric that use different aggregate functions : e.g., Maximum Return, Mean Return and Normalized Return are labeled Return (cite paper) and we created another annotation for the aggregate function.
% \item All metrics that refer to the same formulation across papers have been standardized (e.g., rounds from \cite{ding2020IIC} has been changed to episodes). Same for the algorithms that slightly differ from the baseline algorithm but have different namings (e.g., one example here and provide details (table siddarth prepared)in the supplemental material). Also, environment scenarios that have different naming but refers to the same setting have been unified (e.g., ).
\item We omit ablation studies presented in papers and only log the main algorithm results since we opt to focus primarily on reported algorithmic performance. 
\item We record whether results from previous work has been cited and not reproduced.
\item We record whether any kind of statistical significance testing for the difference between reported metric scores between algorithms has been performed. Unfortunately, only one paper did mention that they perform significance testing (cite paper). % double check
\item We recorded whether the data in a paper is presented using plots or in tabular form. When data is only provided by using plots, we record the final value for a given metric. We also still report the number of seeds, aggregate function and measure of spread as given by the authors. Since we do not have access to the exact confidence bounds for the data read from plots, we add 5\% confidence interval value in order to compare algorithm performance accross papers.
\end{enumerate}

By logging some metrics according to A7, we still highlight that the authors do give a measure of spread but we know that: we are not using the measure of spread mentioned in the paper and that we are reporting the final value as given in the plots.

Our annotations are available as supplemental material for this paper. To benefit the research community from our work and keep track of the evolution of  MARL research, we make our annotated-dataset available online.  

% \begin{comment}
% In this section, we outline findings based on our analysis of the 114 papers and provide them in the manner in which an experiment should be conducted.
% \end{comment}
\subsection{Algorithms}
% \begin{comment}
% In this section:
% Distinguish between Independent Learning and CTDE
% Provide analysis of each type
% Analysis of the most used algorithms 
% \end{comment}
\begin{table}[hbt!]
  \caption{Most used algorithms}
  \label{sample-table}
  \centering
  \begin{tabular}{lllll}
    \toprule
    Algorithms & Type of agent & CTDE & On-/Off-policy  & Mentions  \\
    \midrule
    QMIX \citep{rashid2018qmix} & Value-based  & Yes & Off & 57 \\
    MADDPG \citep{lowe2017multi} & Actor-critic  & Yes & Off & 37\\
    VDN \citep{sunehag2017value} & Value-based & Yes & Off & 33\\
    IQL \citep{} & Value-based  & No & Off & 31\\
    COMA \citep{foerster2018counterfactual} & Actor-critic  & Yes & On & 25\\
    MAPPO \citep{yu2021surprising} & Actor-critic  & Yes & On & 19\\
    QTRAN \citep{son2019qtran} & Value-based  & Yes & Off & 13\\
    QPLEX \citep{wang2020qplex} & Value-based  & Yes & Off & 12\\
    CommNet \citep{sukhbaatar2016learning} & Policy optimization  &  &  & 10\\
    IPPO \citep{} & Actor-critic  & No & On & 08\\
    IAC \citep{} & Actor-critic  & No & On & 08\\
    \bottomrule
  \end{tabular}
\end{table}
\subsubsection{Overview}
\textbf{Independent Learning (IL): } naively extends SARL to the multi-agent space. Agents learn a independent policy based on their own local observations and, in the cooperative case learn a policy based on a shared global reward. This method of learning has poor convergence guarantees as the learning of other agents make the environment seem non-stationary from the egocentric perspective of each other agent.

% % \begin{comment}
% % For example, IQL, an independent learning algorithm, perform well in simple tasks from SMAC such as in (scenario), where IQL has attained (value) over (number of papers) papers, allowing it to compete against CTDE algorithms, whereas in a more complex scenarios like (senario 2), it perform very poorly with (value). 
% % \end{comment}

% % \begin{comment}
% % In cooperative environments, IL algorithms perform well in basic tasks that do not require coordination between agents (full observable also one of the reasons but we need to verify it), such as in (scenario), where IQL has attained (value) over (number of papers) papers, allowing it to compete against CTDE algorithms. However, in complex or partially observable settings, IL algorithms frequently perform poorly, as in (scenario), where they froze in u\% whereas k\% of CTDE algorithms surpassed v\%. Nevertheless, we find (number papers) use IL algorithms as baseline for their experiments where u\% evaluated in (environment name) (we may have takeaway here like the features of the env...) (the main reason for this low performance)
% % \end{comment}

\textbf{Centralised Training Decentralised Execution (CTDE):} 
much like IL, CTDE learns a decentralised policy where agents act based on local observations however, in the CTDE paradigm we can make use of additional information that is normally not available to ILs during execution.Typically this is done using a \textit{centralised-critic} which has access to the ground truth state information or open communication channels with the ILs. The \textit{centralised-critic} is only used during training time which aids in finding better agent polices during training time without increasing computational overheads during execution time. 
% % \begin{comment}
% % "In contrast to IL, CTDE allows sharing of information during training, while policies are only conditioned on the agents’ local observations enabling decentralised execution."(we need to make something similar to this definition)\\
% % We tackle a diversity of CTDE algorithms, with k\% of the algorithms reported in our analysis being CTDE.
% % \end{comment}

% % We also need to discuss parameters sharing 

\subsubsection{Benchmark algorithms}
It is natural for a researcher to want to evaluate the performance of a novel algorithm against some relevant baselines in order to verify whether it is leading improvements on current research. We seek to provide a set of baseline algorithms to be considered that are well studied and provide competitive baselines in existing literature. The baselines must also cover both the CTDE and IL paradigm for cooperative MARL and Policy Gradient (PG) and Q-learning based methods. To meet these requirements we select Qmix \citep{rashid2018qmix}, MADDPG \citep{lowe2017multi}, COMA \citep{foerster2018counterfactual}, IQL \citep{tampuu2015multiagent} and MAPPO \citep{yu2021surprising}. Qmix is selected as it introduced the concept of monotonic value-decomposition which formed the basis for the development of many of the recent algorithmic developments and, as shown by \citep{hu2021rethinking} finetuned implementations of Qmix can still outperform newer methods that attempt to improve upon the original work (add citation). We recommend MADPPG since, at the time of writing, it is the most widely cited MARL algorithm paper with 2070 citation at the time of writing. MADDPG also serves as a clear baseline for algorithms that are used particularly on mixed and competitive tasks. Although MADDPG was introduced as an algorithm to be used on environments with continuous action spaces, the algorithm may also be adapted to the discrete case. We recommend CommNet since it is a widely used algorithm used in scenarios which require agent communication in order to find optimal solutions. Furthermore we recommend MAPPO due to recent work illustrating it's effectiveness in cooperative MARL tasks \citep{yu2021surprising} and COMA since it is a widely used actor-critic algorithm. Moreover, each of the algorithms mentioned have open sourced code implementations available \citep{samvelyan19smac, papoudakis2021benchmarking, hu2021rethinking} which serve to decrease the amount of time researchers have to spend on implementing baselines to evaluate against. 

% % Don't have an example of a CommNet implemetation. 
In our analysis, we examine n algorithms where u\% used only once over the 114 papers. In this section, we focus on revealing insights from our analysis about the most relevant algorithms that we can consider them as benchmark algorithm (baselines), which are summarized in Table 1.
% % discuss why these 5 algorithms are chosen and why we recommend them for a researcher that wants to test their novel algorithm 

\textbf{QMIX:} is a value-based algorithm introduced by \citep{rashid2018qmix} following on from the success of VDN \citep{sunehag2017value} in cooperative MARL tasks. Similarly to VDN, QMIX makes use of a factorized joint Q-value function to train all agents. What differentiates QMIX from VDN is that individual agents' Q-values are joined using a mixing network, which is a fully connected MLP, instead of only summing them. Furthermore, the mixing network is constrained to having only positive weights leading to a monotonic factorisation of individual agent Q-values and also conditions on the global environment state. QMIX follows the CTDE training paradigm and also makes use of recurrent neural networks for individual agent value functions by default. This enables agents to learn joint policies in partially observable settings. The initial performance of QMIX was illustrated by \citep{rashid2018qmix} on the SMAC benchmark.
% % Finding in the analysis for algorithm use
% In our analysis QMIX, variants of QMIX and algorithms building on QMIX feature most prominently in the mmm2 (13), 3s5z (12), 2s3z (11) and 5m vs 6m (9) SMAC scenarios. With numbers in parenthesis denoting the number of papers in which a QMIX variant is benchmarked on a particular scenario. Notably, all of these scanrios are cooperative scenarios; which is to be expencted since QMIX is inherently developed to be used in the cooperative MARL setting.

\textbf{CommNet:} 
% %(Brief algorithm summary)
CommNet \citep{sukhbaatar2016learning} seeks to address the issue of effective agent communication in partially observable cooperative settings. What differentiated CommNet from previous communication works is that the communication protocol between agents is not fixed, but instead learnt as a neural model alongside agent training as agent communication is modeled using a continuous, differentiable vector which is output by each agent. 

% We find that CommNET is used most widely on the TrafficJunction suite of environments, which could be considered one of the most widely used communications benchmarks for MARL. We also find that CommNET is used by 2 papers on the 10m vs 13z, 15w vs 17w and 15 vs 16m SMAC scenarios.

\textbf{Multi-Agent Deep Deterministic Policy Gradient (MADDPG): } introduced by \citep{lowe2017multi}, is a multi-agent extension of the DDPG algorithm introduced by \citep{lillicrap2015continuous}. MADDPG is an off-policy  actor-critic type algorithm and, by default, each agent has a unique policy network and Q-value critic network. Each agent's policy is only allowed to condition on an agent's partial observation of the full environment state while, during training time, each critic conditions on the actions selected by all agents' policy networks.MADDPG makes use of standard MLPs for both the agent policy and critic networks but variations of MADDPG exist which make use of  neural networks (RNNs) for agent policies. Similarly, variations of MADDPG exist which makes use of weight sharing across agent networks to aid in speedups of algorithm training. An advantage of MADDPG is that hte algorithm is inherently applicable to both competitive, cooperative and mixed environments. This versatility is displayed in the seminal paper by \citep{lowe2017multi}.\\ %% citations needed here. 
In our analysis, MADPPG is most widely used for benchmarking on the multi-agent particle environment suite (MPE) with the algorithm being most widely used on the Spread (13), Speaker-listener (8), Predator-prey (7) and reference (6) scenarios. 

\textbf{Multi-Agent Proximal Policy Optimization (MAPPO):} is a multi-agent extension to the single-agent Proximal Policy Optimization (PPO) algorithm and mentioned explicitly by \citep{yu2021surprising}. Similarly to PPO, MAPPO makes use of a value function, conditioned on the global environment state, to serve as a baseline leading to reduced variance in policy-gradient optimization. Furthermore, MAPPO may be implemented in the CTDE or IL paradigms depending on whether the value function is allowed to condition on some representation of the global environment state or only on an agent's local observation of the environment.
% % here we are considering corridor and corridor_sc4.10 to be totally separate environments 
% In our analysis, we find that MAPPO is used an equal amount of times (4) on the corridor, 3s5z vs 3s6z, 3s5z and 5m vs 6m SMAC scenarios as well as on the spread MPE scenario. Notably all these scenarios are cooperative. 

\textbf{Counterfactual Multi-Agent Policy Gradients (COMA):}
COMA \citep{foerster2018counterfactual} is an actor-critic algorithm the makes use of the CTDE paradigm by using a centralized critic, which is allowed to condition on the full environment state, with decentralized actors. This centralized critic is used during training time only and foregone at execution time. The core contribution of COMA is through addressing the agent credit assignment issue in MARL by utilizing a \textit{counterfactual} advantage function that is unique to each agent. % maybe add some information about the advantage function. 

In our analysis we find that COMA is used most frequently in the 3s5z (5), 2s vs 1sc (4), 2s3z (4) and the 1c5s5z (4) SMAC scenarios. 

% %% it could be well worth restating this in the absence of SMAC since it dominates most of our results. 

\subsection{Environments}
The choice of the environment for an algorithm designer is a critical task, considering the fact that each environment has its own challenges, and its own sets of rules, parameters, and even \emph{its own metrics} (e.g. In SMAC, Win Rate is used in 28 papers out of 32, but in MPE, it is used in only one paper out of the 29 papers that use MPE.). All these circumstances can work in the algorithm's favor (alg A reach v in E1) or in its misfortune (alg A reach v2 in E2). In this section, we try to illustrate the characteristics of the existing environments and investigate the relative position of each of them in the field.
\subsubsection{Overview}
\begin{table}[hbt!]
  \caption{Most applicable parameters in each Environment}
  \label{sample-table1}
  \centering
  \makebox[1 \textwidth][c]{ 
  \begin{tabular}{lllllll}
    \toprule
    Environment & Metric & R. Seed & Aggregate Function & Independent variable & Popular Task & Env. Mentions \\
    \midrule
    SMAC\cite{} & Win Rate (88.3\%) & 5 (46\%) & Median (68.1\%) & Timestep (97.3\%) & 3s5z & 32 \\
    MPE\cite{} & Reward (48.9\%) & 3 (41.4\%) & Mean (89.9\%) & Episode (48\%) & Predator-Prey & 31\\
    Matrix Games\cite{} & Return (100\%) & 5 (71\%) & Mean (100\%) & Timestep (98.7\%) & - & 9\\
    MazeBase\cite{} & Win Rate (94.3\%) & 5 (74.6\%) & Mean (100\%) & Episode (44.1\%) & Traffic Junction & 8 \\
    \bottomrule
  \end{tabular}}
\end{table}
In our study, we differentiate between environment and task by using the term "environment" to refer to a simulator with various scenarios with different aims and parameters, whilst "task" refers to a specific scenario within an environment. We look over 29 environments that are composed of 155 tasks in total. In this part, we are primarily interested in disclosing insights from our investigation concerning the most applicable settings that are summarized in Table 2.

\textbf{StarCraft Multi-Agent Challenge (SMAC):} is a partially observable environment, with a diverse set of sophisticated micro-actions that enable the learning of complex interactions amongst collaborating agents, the fundamental concept of SMAC is a team of agents battling against another unit.SMAC is the most widely used environment in our analysis, since it is employed as the experimental environment in 32 of the papers and in 46.4\% of the data collected. This finding is not surprising given that we record 36 scenarios with varying scales of difficulty. Many authors agree that SMAC offers a fair comparisons of different algorithms since it provides an open-source Python-based implementation of numerous fundamental algorithms.

\textbf{Multi-Agent Particle Environment (MPE):} is an environment that can be fully or partially observable, cooperative or competitive, and allow communication within some of its tasks. In this environment, to attain various purposes, the agents primarily interact with the landmark and other entities. We discover that 31 of the 65 papers employ MPE for algorithm testing, accounting for 21\% of the data collected. MPE, like SMAC, is a diversified environment with 21 tasks; nevertheless, we observe a disparity in their utilization, with 20.3\%of cases utilizing Predator and Prey, followed by Spread presenting 20\% of MPE collected data.

\subsection{Annotations}
\subsubsection{Environments' annotations}
\begin{itemize}
    \item All SMAC win rates are reported as percentages (out of 100) and not probabilities (out of 1).
    \item When we move from a cooperative environment to a mixed one like predator-prey and the authors record the reward for the predator alone and then the prey alone, we change the environment name to predator-prey-separate and we add in the metric settings whether we are currently recording the predator or the prey reward.
\end{itemize}

\subsubsection{Algorithms' annotations}
\begin{table}[hbt!]
  \caption{Algorithms' annotations}
  \label{sample-table}
  \centering
  \begin{tabular}{lll}
    \toprule
    Name from paper & Standard name &  Our interpretation  \\
    \midrule
    IAC-V\cite{} & IAC  & They are the same. The COMA paper used IAC-V and IAC-Q to test if the Q learning of Value based critic impact performance. \\
    IDL\cite{} & IQL  &  An algorithm is listed as IDL. Should probably be IQL since that's what they use in the graphs. \\
    PSMADDPG\cite{} & MADDPG  & PSMADDPG can be considered an implementation variant of MADDPG.\\
    A3C\cite{} & IAC  & A3C is a method for parallising the AAC/A2C algorithm. I think we can just consider this as an IAC implementation.\\
    A2C\cite{} & IAC  & Need to look at implementation. They use A2C which should just be IAC in the MARL case if they're just using a naïve implementation.\\
    MADQN\cite{} & IQL  & Old paper using MADQN. We should change to IQL\\
    Naïve critic\cite{} & Central-V  & Naïve critic is the same as central-v.\\
    MAPPO-shared\cite{} & MAPPO  &  MAPPO-shared is MAPPO with parameter sharing.\\
    MAPPO-FP\cite{} & MAPPO with options  & MAPPO-FP is the version of PPO using the augmented state space from the MAPPO paper.\\
    MAPPO-AS\cite{} & MAPPO with options  &  MAPPO-AS is an augmented MAPPO variant and is good as a raw performance test.\\
    MADR\cite{} & MADDPG  & MADR seems to be MADDPG with recurrent layers. \\
    DDPG\cite{} & IDDPG  & Old paper uses DDPG. Can change to IDDPG so we have consistency between all the independent learning algorithms. \\
    DQN\cite{} & IQL  & Old paper uses DQN. Can change to IQL for consistency. \\
    \bottomrule
  \end{tabular}
\end{table}
